# Supplementary material for: The Many Faces of Robustness: A Critical Analysis of Out-of-Distribution Generalization
Source: arXiv:2006.16241 source file (2021-07-24)
Supplement: Supplementary file 1 [file supplementary.tex]

\documentclass[10pt,twocolumn,letterpaper]{article}

\usepackage{iccv}
\usepackage{times}
\usepackage{epsfig}
\usepackage{graphicx}
\usepackage{amsmath}
\usepackage{amssymb}

\usepackage{listings}
\usepackage{xcolor}

\definecolor{codegreen}{rgb}{0,0.6,0}
\definecolor{codegray}{rgb}{0.5,0.5,0.5}
\definecolor{codepurple}{rgb}{0.58,0,0.82}
\definecolor{backcolour}{rgb}{0.97, 0.97, 0.97}

\lstdefinestyle{mystyle}{
    backgroundcolor=\color{white},   
    commentstyle=\color{codegray},
    keywordstyle=\color{codeblue2},
    numberstyle=\tiny\color{codegray},
    stringstyle=\color{codeblue},
    basicstyle=\fontsize{9pt}{9.5pt}\fontfamily{lmtt}\selectfont,
    breakatwhitespace=false,         
    breaklines=true,                 
    captionpos=b,                    
    keepspaces=true,                 
    numbers=left,                    
    numbersep=12pt,                  
    showspaces=false,                
    showstringspaces=false,
    showtabs=false,                  
    tabsize=2,
    framexleftmargin=20pt,
    framextopmargin=10pt,
    framesep=30pt,
}

\lstset{style=mystyle}

\usepackage[utf8]{inputenc} %
\usepackage[T1]{fontenc}    %
\usepackage{amsfonts}       %
\usepackage{nicefrac}       %
\usepackage{microtype}      %

\usepackage{epsfig}
\usepackage{graphicx}
\usepackage{xcolor}
\usepackage{amsmath}
\usepackage{amssymb}
\usepackage{subcaption}
\usepackage{textcomp}
\usepackage{gensymb}
\usepackage{mathtools}
\usepackage{amssymb}
\usepackage{wrapfig}
\usepackage{lipsum}
\usepackage{diagbox}

\usepackage{booktabs}
\usepackage{float}
\usepackage{hhline}
\usepackage{tabularx}
\newcolumntype{Y}{>{\centering\arraybackslash}X}
\newcolumntype{L}{>{\raggedright\arraybackslash}X}
\newcolumntype{s}{>{\hsize=.8\hsize}Y}
\newcolumntype{t}{>{\hsize=.6\hsize}Y}
\newcolumntype{?}{!{\vrule width 1pt}}
\usepackage{multirow}
\restylefloat{table}
\usepackage{makecell}

\usepackage{arydshln}
\usepackage{dsfont}

\usepackage{letltxmacro}
\makeatletter
\let\oldr@@t\r@@t
\def\r@@t#1#2{%
	\setbox0=\hbox{$\oldr@@t#1{#2\,}$}\dimen0=\ht0
	\advance\dimen0-0.2\ht0
	\setbox2=\hbox{\vrule height\ht0 depth -\dimen0}%
	{\box0\lower0.4pt\box2}}
\LetLtxMacro{\oldsqrt}{\sqrt}
\renewcommand*{\sqrt}[2][\ ]{\oldsqrt[#1]{#2}}
\makeatother

\makeatletter
\newcommand{\thickhline}{%
	\noalign {\ifnum 0=`}\fi \hrule height 1pt
	\futurelet \reserved@a \@xhline
}
\newcolumntype{"}{@{\hskip\tabcolsep\vrule width 1pt\hskip\tabcolsep}}
\makeatother

\makeatletter
\newcommand*{\defeq}{\mathrel{\rlap{%
			\raisebox{0.3ex}{$\m@th\cdot$}}%
		\raisebox{-0.3ex}{$\m@th\cdot$}}%
	=}
\makeatother

\usepackage[pagebackref=true,breaklinks=true,letterpaper=true,colorlinks,bookmarks=false]{hyperref}

\ificcvfinal\pagestyle{empty}\fi

\usepackage{multicol}
\usepackage{appendix}
\usepackage{cleveref}
\crefname{appsec}{Appendix}{Appendices}
\usepackage{enumitem}

\newcommand{\reviewer}[3]{
	\expandafter\newcommand\csname #1\endcsname[1]{
		\textcolor{#3}{[#2: ##1]}
	}
}
\reviewer{norman}{Norman}{green}
\definecolor{neonpurple}{rgb}{0.3,0,1}
\reviewer{dan}{Dan}{neonpurple}
\reviewer{justin}{Justin}{blue}

\title{The Many Faces of Robustness: A Critical Analysis of\\Out-of-Distribution Generalization}

\author{%
    Dan Hendrycks$^1$ \And Steven Basart$^2$\thanks{Equal contribution. \qquad Code is available at \url{https://github.com/hendrycks/imagenet-r}} \And Norman Mu$^{1}$\footnotemark[1] \And Saurav Kadavath$^1$ \And Frank Wang$^3$ \And Evan Dorundo$^3$ \And Rahul Desai$^1$ \And Tyler Zhu$^1$ \And Samyak Parajuli$^1$ \And Mike Guo$^1$
    \AND Dawn Song$^1$ \And Jacob Steinhardt$^1$ \And Justin Gilmer$^3$
    \AND\textnormal{$^1$UC Berkeley} \And \textnormal{$^2$UChicago} \And \textnormal{$^3$Google}
}

\begin{document}

\title{Scaling Out-of-Distribution Detection for Real-World Settings\\Supplementary Material}

\author{First Author\\
Institution1\\
Institution1 address\\
{\tt\small firstauthor@i1.org}
\and
Second Author\\
Institution2\\
First line of institution2 address\\
{\tt\small secondauthor@i2.org}
}

\maketitle
\ificcvfinal\thispagestyle{empty}\fi

\appendix

\input{sections/7-appendix}

\newpage
{\small
\bibliographystyle{ieee_fullname}
\bibliography{main}
}

\end{document}
